# Supplementary material for: Non-Clicks Mean Irrelevant? Propensity Ratio Scoring As a Correction
Source: arXiv:2005.08480 source file (2021-11-14)
Supplement: Supplementary file 1 [file appendix.tex]

The insight of identifying truly irrelvant documents in non-clicked documents comes from the decomposition of click data in Figure \ref{fig:clickdata}. In a noise-free setting if the relevance label of a document is observed (the first column in Figure \ref{fig:clickdata}), click is equivalent to relevance, i.e., $o_q(x_i)=1 \rightarrow [c_q(x_i)=r_q(x_i)]$. Consequently, if a document is observed and non-clicked, it is irrelevant, i.e., $[o_q(x_i)=1 \wedge c_q(x_i)=0] \rightarrow r_q(x_i)=0$
%. In other words, if a document is non-clicked but observed, it is irrelevant 
(the I\&O part in Figure \ref{fig:clickdata}). Therefore, \textit{the problem of identifying truly irrelevant documents from non-clicked ones is mapped to finding the observed documents in the non-clicked ones.}

\textbf{Our original claims (wrong)}: for a non-clicked document $x_j$, although we do not know the true observation $o_q(x_j)$, we can still estimate its observation propensity $o_q(x_j)\sim P(o_q(x_j)=1|\tilde\pi_q)$ \cite{Craswell2008clickpositionbias,wang2018pbe,Agarwal2019EPB}. By weighing the loss on each non-clicked document with its observation propensity, in expectation we restrict the loss on non-clicked documents to those that are non-clicked but observed, which are truly irrelevant:
\begin{align}
\label{eq:PNS-expectation}
    &\sum_{x_j:c_q(x_j)=0}\Omega(x_j|\pi_q)\cdot P(o_q(x_j)=1|\tilde\pi_q) \\\nonumber
    =&\; E_{o_q}\Big[\mathop{\sum_{x_j:o_q(x_j)=1}}_{\wedge c_q(x_j)=0}\Omega(x_j|\pi_q)\Big]
    =\; E_{o_q}\Big[\mathop{\sum_{x_j:o_q(x_j)=1}}_{\wedge r_q(x_j)=0}\Omega(x_j|\pi_q)\Big]\nonumber
\end{align}
where $\Omega(\cdot)$ represents any general loss on $x_j$. The last step is obtained by: $[o_q(x_j)=1 \wedge c_q(x_j)=0] \rightarrow r_q(x_j)=0$ (see Figure \ref{fig:clickdata}). We refer to this weighting on non-cliked documents as the Propensity-weighted Negative Samples (PNS). This weighting scheme is also intuitive: if a document in the presented rank list is not clicked but very likely observed, there should be a good chance that it is irrelevant. 

\textbf{Correction}: In the original claims, we implicitly assumed click and observation are independent, and thus we can directly apply the observation propensity weights to both clicks and non-clicks. However, this is not true. The main reason is that in noise-free setting, if a relevant document is non-clicked, it must be unobserved, and thus the observation probability is $P(o_q(x_j)=1|c_q(x_j)=0,r_q(x_j)=1) = 0$. So if we are still using the propensity for weighting relevant documents in non-clicked documents, we actually cannot remove the relevant documents from non-clicks in expectation:
\begin{align}
\label{eq:corrected-expectation}
    &\sum_{x_j:c_q(x_j)=0}\Omega(x_j|\pi_q)\cdot P(o_q(x_j)=1|\tilde\pi_q) \\\nonumber
    =&\; \sum_{x_j:r_q(x_j)=0}\Omega(x_j|\pi_q)\cdot P(o_q(x_j)=1|\tilde\pi_q) + \mathop{\sum_{x_j:r_q(x_j)=1}}_{\wedge o_q(x_j)=0}\Omega(x_j|\pi_q)\cdot P(o_q(x_j)=1|\tilde\pi_q) \\\nonumber 
    =&\; E_{o_q}\Big[\mathop{\sum_{x_j:o_q(x_j)=1}}_{\wedge r_q(x_j)=0}\Omega(x_j|\pi_q)\Big] + \mathop{\sum_{x_j:r_q(x_j)=1}}_{\wedge o_q(x_j)=0}\Omega(x_j|\pi_q)\cdot P(o_q(x_j)=1|\tilde\pi_q)
\end{align}
where the second term is the extra loss from the relevant documents in non-clicked documents that PRS cannot remove. Ideally, if we use the observation probability conditioned on the clicks, the second term should be zero, since if a non-clicked relevant document has zero observation probability. Unfortunately, we are not able to directly identify the relevant documents in non-clicked documents, and thus can only apply propensity weights on all non-clicked documents.  

\textbf{Can we really solve this problem?} I am afraid not. In our discussions with Hongbo and Jingyue, they mentioned that we might be able to estimate the probability of a non-click document being the irrelevant document. The logic is as follows. For each position, we can count the number of clicked documents, say $n_c$, and with the propensity at this position, we can estimate the number of all relevant documents $n_r$. Then based on the total number of documents presented at this position $n$, we can get the probability of a non-clicked document $x_j$ being an irrelevant document as $P(r(x_j)=0|c(x_j)=0)=\frac{n-n_r}{n-n_c}$. However, this is totally data-dependent, which means such probabilities depend on the specific click data as well as the document set (the number of relevant document and irrelevant document). Thus for each new click data, we need to estimate such probabilities for each position all over again. 

Besides, I also doubt the meaning of using such probabilities for weighting the loss terms. Specifically, we need to assume the counts can give us the correct estimate of the probability $P(r(x_j)=0|c(x_j)=0)$ and it is the same for all queries. I am not sure if this is a solid argument, and if this method is practical.

\textbf{How good is PRS?}
As we can see, the second term in Eq~\eqref{eq:corrected-expectation} is the extra term on relevant documents in our previous derivation. Without applying any weights, this term would be $\sum_{x_j:r_q(x_j)=1\wedge o_q(x_j)=0}\Omega(x_j|\pi_q)$. But after applying the propensity weights, we can reduce this term by at least $\max\{p_2, \dots, p_m\}$, where $p_k$ is the propensity at position $k$ and $m$ is the maximum length of the document list. If we assume the exponentially decaying propensity model in Section 5.2 with $\eta=1$, the relevant documents at the first position must be clicked. Then the largest propensity in the following positions will be $0.5$, which means we reduced the extra term by 50\% after propensity weighting. However, in general, we do not expect too many relevant documents being missed at position 2, and thus this term should be reduced much more than 50\% in practice, depending on the positions of non-clicked relevant documents. Therefore we may do some simulation based experiments to show that PRS can already achieve good performance compared to directly eliminating the relevant documents from the non-clicked documents.
